# Supplementary material for: A Mechanism for Producing Aligned Latent Spaces with Autoencoders
Source: arXiv:2106.15456 source file (2021-06-29)
Supplement: Supplementary file 9 [file appendix_alignment_intuition.tex]

% \begin{lemma}
% \label{lemma: Alignment Intuition}
%     Let $B \in \mathbb{R}^{h \times d}$ be a positive semi-definite matrix with singular value decomposition $B=U\Sigma_BV^T$, where $\sigma_i$ and $v_i$ are the i\textsuperscript{th} singular value and singular vector of $B$. Let $q_1, q_2 \in \mathbb{R}^d$ be unit vectors and let $\cos \theta_i^{(j)} = q_j^Tv_i$.  Then,
%     $$\cos \theta' = \frac{(Bq_1)^T Bq_2}{\|Bq_1\|_2\|B q_2\|_2} = \frac{
%         \sum_{i=1}^d \sigma_i^2 \cos \theta_i^{(1)} \cos \theta_i^{(2)}
%         }{\sqrt{
%             \left(\sum_{i=1}^d \sigma_i^2 (\cos \theta_i^{(1)})^2\right)
%             \left(\sum_{i=1}^d \sigma_i^2 (\cos \theta_i^{(2)})^2\right)
%         }}$$
% \end{lemma}
\begin{proof}
We note that:
\begin{align*}
    (Bq_1)^T(Bq_2) &= q_1^T B^T B q_2 \\
    &= q_1^T V \Sigma B^2 V^T q_2\\
    &= \sum_{i=1}^d \sigma_i^2 (q_1^Tv_1) (q_2^Tv_2)\\
    &= \sum_{i=1}^d \sigma_i^2 \cos \theta_i^{(1)} \cos \theta_i^{(2)}
    ||Bq_j||_2 = \sqrt{q_j^T B^T B q_j}\\
    &= \sqrt{\sum_{i=1}^d  \sigma_i^2 (\cos \theta_i^{(j)})^2}.
\end{align*}
We thus have:
$$\cos(Bq_1, Bq_2)= \frac{(Bq_1)^T Bq_2}{\|Bq_1\|_2\|B q_2\|_2} = \frac{
    \sum_{i=1}^d \sigma_i^2 \cos (q_1, v_i) \cos(q_2, v_i)
    }{\sqrt{
        \left(\sum_{i=1}^d \sigma_i^2 (\cos (q_1, v_i)^2\right)
        \left(\sum_{i=1}^d \sigma_i^2 (\cos (q_2, v_i)^2\right)
    }}.$$
\end{proof}
