# Supplementary material for: A Mechanism for Producing Aligned Latent Spaces with Autoencoders
Source: arXiv:2106.15456 source file (2021-06-29)
Supplement: Supplementary file 12 [file stretching_lemma_appendix.tex]

\begin{proof}
Let $x_i^{(j)}$ be the the ith example from $X_1$ and $x_i^{(2)}$ be the ith example from $X_2$. Then we note that 
$$\frac{1}{n}XX^T = \frac{1}{n}\sum_{i=1}^n \begin{bmatrix} x_i^{(1)} & x_i^{(2)} ... & x_i^{(m)}\end{bmatrix}  \begin{bmatrix} x_i^{(1)} & x_i^{(2)} ... & x_i^{(m)}\end{bmatrix}^T.$$

Let $x = \begin{bmatrix} x^{(1)} &  x^{(2)}...& x^{(m)}\end{bmatrix}, x\in \mathcal{R}^{d \times m}$ where $x_i \sim \mathcal{N}(\mu_i, \Sigma_i)$. Then by the strong law of large numbers, as n tends to infinity, we have that:
$$B^{(0)} = \frac{1}{n}XX^T \xrightarrow{a.s} \EE[xx^T].$$

Furthermore
\begin{align*}
    \EE[xx^T] &= \sum_{i=1}^m \EE[x^{(i)}x^{(i)^T}]\\
    &= \sum_{i=1}^m \Sigma_i + \mu_i\mu_i^T.
\end{align*}
Moreover $\EE[xx^T] = \EE[\frac{1}{n}XX^T]$. We can then plug in the relevant values for $\Sigma_i$:
\begin{align*}
     \EE[xx^T] &= \sum_{i=1}^m D_i + \mu_i \sum_{j=1}^m \mu_j^T\\
     &=  cI + \left(\sum_{j=1}^m \mu_j\right)\left(\sum_{j=1}^m \mu_j\right)^T.
\end{align*}

\end{proof}
